# Supplementary material for: SoK: The Faults in our Graph Benchmarks
Source: arXiv:2404.00766 source file (2024-03-31)
Supplement: Supplementary file 1 [file appendix.tex]

\appendix
